# Supplementary material for: HiNER: A Large Hindi Named Entity Recognition Dataset
Source: arXiv:2204.13743 source file (2022-04-28)
Supplement: Supplementary file 1 [file 6.Appendix.tex]

\begin{table*}[ht!]
\centering
\resizebox{\textwidth}{!}{%
\begin{tabular}{lrrrrr}
\toprule
{} & \multicolumn{1}{c}{\textbf{indic-bert}} & \multicolumn{1}{c}{\textbf{mBERT}} & \multicolumn{1}{c}{\textbf{muril}} & \multicolumn{1}{c}{\textbf{xlm-roberta-base}} & \multicolumn{1}{c}{\textbf{xlm-roberta-large}} \\
\midrule
Location & 68.32 $\pm$ 1.11 & 66.22 $\pm$ 0.93 & 68.51 $\pm$ 0.74 & 69.78 $\pm$ 0.66 & 70.99 $\pm$ 0.40 \\
Organization & 34.02 $\pm$ 4.32 & 38.14 $\pm$ 2.56 & 0.00 $\pm$ 0.00 & 42.10 $\pm$ 2.86 & 43.41 $\pm$ 2.05 \\
Person & 61.53 $\pm$ 0.66 & 61.36 $\pm$ 0.74 & 61.54 $\pm$ 3.55 & 64.90 $\pm$ 1.39 & 65.95 $\pm$ 0.55 \\
\midrule
Micro & 62.79 $\pm$ 0.68 & 62.14 $\pm$ 0.59 & 62.58 $\pm$ 2.44 & 65.63 $\pm$ 0.76 & 66.75 $\pm$ 0.30 \\
Macro & 54.62 $\pm$ 1.88 & 55.24 $\pm$ 0.90 & 43.35 $\pm$ 1.36 & 58.93 $\pm$ 1.08 & 60.11 $\pm$ 0.74 \\
Weighted & 62.42 $\pm$ 0.78 & 61.85 $\pm$ 0.54 & 61.08 $\pm$ 2.49 & 65.42 $\pm$ 0.82 & 66.52 $\pm$ 0.32 \\
\bottomrule
\end{tabular}%
}
\caption{Test Set F1-Score of various pre-trained LMs on FIRE 2014 dataset (Collapsed). This table reports mean F1-score and its standard deviation over 5 runs.}
\label{tab:resultsFIRE}
\end{table*}

% \hbox{}\newpage

\begin{table}[!htb]
\begin{tabular}{@{}lrrrr@{}}
\toprule
 & \multicolumn{1}{c}{\textbf{Train}} & \multicolumn{1}{c}{\textbf{Dev}} & \multicolumn{1}{c}{\textbf{Test}} & \multicolumn{1}{c}{\textbf{Total}} \\ \midrule
Location & 1711 & 203 & 354 & 2268 \\
Person & 1144 & 191 & 777 & 2112 \\
Organization & 96 & 25 & 49 & 170 \\
\midrule
\textbf{Total} & 2951 & 419 & 1180 & 4550 \\ \bottomrule
\end{tabular}
\caption{Number of Entity mentions in \textit{Train, Dev, Test} splits of \textbf{FIRE 2014} data}
\label{tab:FIRE2014stats}
\end{table}

\section{Appendix}
\label{sec:appendix}

Table \ref{tab:FIRE2014stats} reports FIRE 2014 NER data statistics for Hindi. Table \ref{tab:resultsFIRE} reports detailed results of training and testing on FIRE 2014 data using various pre-trained language models.
